# Supplementary material for: Farthest Streamline Sampling for the Uniform Distribution of Forearm Muscle Fiber Tracts from Diffusion Tensor Imaging
Source: arXiv:2306.13969 ancillary file (2023-06-24)
Supplement: Supplementary file 1 [file info_supplementary_materials.pdf]

Supplementary Material 1

Figure. Two-step process of piecewise registration.

Supplementary Material 2

Figure. Registration results of global affine transformation and piecewise registration.

Supplementary Material 3

A movie showing the streamline density maps within the forearm muscles for the three samplings: farthest streamline sampling, two-dimensional sampling, and three-dimensional sampling.

Supplementary Material 4

Table. *In vivo* architectural parameters of human forearm muscles.

Supplementary Material 5

A movie showing the comparison of cadaveric photographs (1) (with permission) and the tractography for supinator. The muscle is rotating around the proximal-distal axis.

Supplementary Material 6

A movie showing the comparison of cadaveric photographs (1) (with permission) and the tractography for flexor carpi ulnaris. The muscle is rotating around the proximal-

distal axis.

Supplementary Material 7

Table. Classification of architectural types in human forearm muscles.

References:

1. Froeling M, Nederveen AJ, Heijtel DFR, et al. Diffusion-tensor MRI reveals the complex muscle architecture of the human forearm. Journal of Magnetic Resonance Imaging 2012;36(1):237-248.
