# Supplementary material for: Farthest Streamline Sampling for the Uniform Distribution of Forearm Muscle Fiber Tracts from Diffusion Tensor Imaging
Source: arXiv:2306.13969 ancillary file (2023-06-24)
Supplement: Supplementary file 2 [file supplementary_material_4_par.pdf]

**Table.** Architecture parameters (mean ± standard deviation) of 17 forearm muscles from 12 healthy individuals (9 males and 3 females, age: 25.3±2.2 years, height: 1.74±0.05 m, body mass: 66.9±7.2 kg, body mass index: 22.0±2.2 kgm$^{-2}$, radius length: 239±16 mm, ulna length: 256±17 mm, forearm circumference: 237±15 mm. Radius length is calculated as the straight-line distance from the styloid process of radius to the lateral humeral epicondyle. Ulna length is measured as the straight-line distance from the styloid process of ulnar to the medial humeral epicondyle. Forearm circumference is the maximum circumference of the forearm). (Abbreviations: fiber length (FL), muscle length (ML), pennation angle (PA), physiological cross-sectional area (PCSA).)

| Muscle | Muscle volume (mm$^3$) | Muscle length (mm) | Fiber length (mm) | FL/ML ratio (–) | PA (deg) | PCSA (mm$^2$) |
|---|---|---|---|---|---|---|
| Anconeus | 6269±2453 | 40±10 | 16±3 | 0.41±0.09 | 9±3 | 396±152 |
| Abductor pollicis longus | 12266±2837 | 108±11 | 39±8 | 0.36±0.07 | 9±2 | 328±103 |
| Extensor carpi radialis brevis | 12149±2825 | 86±17 | 23±5 | 0.27±0.04 | 8±5 | 520±95 |
| Extensor carpi radialis longus | 27492±6041 | 160±28 | 50±11 | 0.32±0.06 | 9±4 | 556±127 |
| Extensor carpi ulnaris | 11816±3119 | 143±12 | 31±12 | 0.21±0.07 | 10±2 | 421±150 |
| Extensor digitorum communis | 19911±4032 | 140±12 | 35±10 | 0.24±0.06 | 9±3 | 605±164 |
| Extensor digiti minimi | 3648±1393 | 95±28 | 23±9 | 0.25±0.06 | 7±2 | 165±63 |

| | | | | | | |
|---|---|---|---|---|---|---|
| Extensor pollicis longus | 6454±2810 | 89±17 | 28±7 | 0.32±0.07 | 9±4 | 225±69 |
| Flexor carpi radialis | 21214±6708 | 136±42 | 48±9 | 0.37±0.09 | 8±2 | 442±113 |
| Flexor carpi ulnaris | 24755±5636 | 173±14 | 41±9 | 0.24±0.04 | 9±2 | 617±172 |
| Flexor digitorum profundus | 68210±11033 | 174±13 | 74±11 | 0.43±0.06 | 7±2 | 941±234 |
| Flexor digitorum superficialis | 52122±12113 | 188±19 | 72±14 | 0.38±0.06 | 7±3 | 732±173 |
| Flexor pollicis longus | 17045±3155 | 149±19 | 44±9 | 0.30±0.05 | 9±3 | 400±99 |
| Palmaris longus | 7789±3505 | 81±20 | 41±12 | 0.50±0.05 | 7±3 | 191±65 |
| Pronator quardratus | 5846±1770 | 36±11 | 22±6 | 0.63±0.08 | 11±3 | 267±62 |
| Pronator teres | 25214±10911 | 84±18 | 35±10 | 0.42±0.06 | 11±2 | 701±217 |
| Supinator | 17129±4388 | 66±15 | 23±2 | 0.32±0.04 | 26±5 | 664±137 |
